# Supplementary material for: Benchmarking the Semi-Stochastic CC(P;Q) Approach for Singlet-Triplet Gaps in Biradicals
Source: arXiv:2205.10707 ancillary file (2022-10-01)
Supplement: Supplementary file 1 [file supplementary-material.pdf]

# Benchmarking the Semi-Stochastic CC($P$;$Q$) Approach for Singlet–Triplet Gaps in Biradicals

Arnab Chakraborty,[1] Stephen H. Yuwono,[1] J. Emiliano Deustua,[1] Jun Shen,[1] and Piotr Piecuch[1,2,a)]
[1)] *Department of Chemistry, Michigan State University, East Lansing, Michigan 48824, USA*
[2)] *Department of Physics and Astronomy, Michigan State University, East Lansing, Michigan 48824, USA*

This document provides the information about the total walker populations at selected propagation times $\tau$ (represented by the numbers of MC iterations) characterizing the various CIQMC runs carried out in this study. The total numbers of walkers used in the $i$-FCIQMC propagations that were needed to generate the CC($P$) and CC($P$;$Q$) energies of the X $^3$B$_1$ and A $^1$A$_1$ states of methylene, as described by the aug-cc-pVTZ basis set, reported in Table I of the main text, can be found in Table S.1. The total numbers of walkers characterizing the $i$-FCIQMC propagations that were used to obtain the CC($P$) and CC($P$;$Q$) energies of the X $^1\Sigma_g^+$ and A $^3\Sigma_u^+$ states of (HFH)$^-$, as described by the 6-31G(d,p) basis set, at selected H–F distances $R_{\text{H-F}}$, reported in Tables II and III of the main text, are shown in Table S.2. The total numbers of walkers characterizing the $i$-FCIQMC propagations for the X $^1$B$_{1g}$ and A $^3$A$_{2g}$ states of cyclobutadiene, as described by the cc-pVDZ basis set, which were needed to determine the CC($P$) and CC($P$;$Q$) data reported in Table V of the main text, can be found in Table S.3. The total numbers of walkers characterizing the $i$-CISDTQ-MC propagations that were used to generate the CC($P$) and CC($P$;$Q$) results for the X $^3$A$_2'$ and A $^1$E$_2'$ states of cyclopentadienyl cation, as described by the cc-pVDZ basis set, reported in Table VI of the main text, can be found in Table S.4. Finally, Table S.5 shows the total numbers of walkers characterizing the $i$-CISDTQ-MC propagations for the X $^3$A$_2'$ and B $^1$A$_1$ states of trimethylenemethane, as described by the cc-pVDZ basis set, which were used to obtain the CC($P$) and CC($P$;$Q$) energies presented in Table VII of the main text.

TABLE S.1. The total numbers of walkers, reported as percentages of the total walker populations at 200000 MC iterations, characterizing the $i$-FCIQMC propagations with $\delta\tau = 0.0001$ a.u. that were needed to generate the CC($P$) and CC($P$;$Q$) results for methylene reported in Table I of the main text.

| MC Iterations | X $^3$B$_1$ | A $^1$A$_1$ |
|---|---|---|
| 0 | 0.02[a] | 0.01[a] |
| 2000 | 0.39 | 0.19 |
| 4000 | 1.00 | 0.51 |
| 6000 | 1.65 | 0.83 |
| 8000 | 2.17 | 1.11 |
| 10000 | 2.58 | 1.35 |
| 20000 | 4.11 | 2.17 |
| 50000 | 7.69 | 4.64 |
| 100000 | 18.59 | 13.13 |
| 150000 | 43.10 | 36.96 |
| 200000 | 100[b] | 100[c] |

[a] The initial walker population, meaning 1500 walkers on the ROHF (X $^3$B$_1$ state) and RHF (A $^1$A$_1$ state) reference determinants.
[b] The total number of walkers at 200000 MC iterations is 6118222.
[c] The total number of walkers at 200000 MC iterations is 14878766.

[a)] Corresponding author; e-mail: piecuch@chemistry.msu.edu.

TABLE S.2. The total numbers of walkers, reported as percentages of the total walker populations at 200000 MC iterations, characterizing the $i$-FCIQMC propagations with $\delta\tau = 0.0001$ a.u. that were needed to generate the CC($P$) and CC($P$;$Q$) results for the X $^1\Sigma_g^+$ and A $^3\Sigma_u^+$ states of $(HFH)^-$ reported in Tables II and III of the main text.

| | $R_{H\text{-}F}$ = 1.50 Å | | $R_{H\text{-}F}$ = 1.75 Å | | $R_{H\text{-}F}$ = 2.00 Å | | $R_{H\text{-}F}$ = 2.50 Å | | $R_{H\text{-}F}$ = 4.00 Å | |
|---|---|---|---|---|---|---|---|---|---|---|
| MC Iterations | X $^1\Sigma_g^+$ | A $^3\Sigma_u^+$ | X $^1\Sigma_g^+$ | A $^3\Sigma_u^+$ | X $^1\Sigma_g^+$ | A $^3\Sigma_u^+$ | X $^1\Sigma_g^+$ | A $^3\Sigma_u^+$ | X $^1\Sigma_g^+$ | A $^3\Sigma_u^+$ |
| 0 | 0.02[a] | 0.09[a] | 0.01[a] | 0.10[a] | 0.01[a] | 0.13[a] | 0.01[a] | 0.24[a] | 0.00[a] | 0.59[a] |
| 2000 | 0.11 | 0.59 | 0.08 | 0.64 | 0.06 | 0.73 | 0.03 | 0.95 | 0.01 | 1.74 |
| 4000 | 0.20 | 1.08 | 0.15 | 1.14 | 0.10 | 1.23 | 0.05 | 1.54 | 0.02 | 2.45 |
| 6000 | 0.27 | 1.36 | 0.19 | 1.46 | 0.13 | 1.59 | 0.07 | 1.86 | 0.02 | 2.97 |
| 8000 | 0.32 | 1.55 | 0.23 | 1.66 | 0.16 | 1.77 | 0.08 | 2.12 | 0.03 | 3.20 |
| 10000 | 0.37 | 1.68 | 0.26 | 1.79 | 0.18 | 1.91 | 0.09 | 2.29 | 0.03 | 3.29 |
| 20000 | 0.55 | 2.19 | 0.40 | 2.38 | 0.28 | 2.46 | 0.15 | 3.03 | 0.06 | 4.09 |
| 50000 | 1.42 | 4.19 | 1.10 | 4.59 | 0.81 | 4.81 | 0.47 | 5.58 | 0.21 | 6.83 |
| 100000 | 6.21 | 12.24 | 5.16 | 12.87 | 4.25 | 13.61 | 2.88 | 15.13 | 1.61 | 16.64 |
| 150000 | 25.44 | 35.16 | 23.37 | 36.28 | 21.01 | 37.71 | 17.11 | 38.88 | 12.45 | 41.09 |
| 200000 | 100[b] | 100[c] | 100[d] | 100[e] | 100[f] | 100[g] | 100[h] | 100[i] | 100[j] | 100[k] |

[a] The initial walker population, meaning 1500 walkers on the RHF (X $^1\Sigma_g^+$ state) and ROHF (A $^3\Sigma_u^+$ state) reference determinants.
[b] The total number of walkers at 200000 MC iterations is 9865967.
[c] The total number of walkers at 200000 MC iterations is 1749699.
[d] The total number of walkers at 200000 MC iterations is 12468454.
[e] The total number of walkers at 200000 MC iterations is 1431689.
[f] The total number of walkers at 200000 MC iterations is 15510033.
[g] The total number of walkers at 200000 MC iterations is 1123676.
[h] The total number of walkers at 200000 MC iterations is 24265207.
[i] The total number of walkers at 200000 MC iterations is 632102.
[j] The total number of walkers at 200000 MC iterations is 50189301.
[k] The total number of walkers at 200000 MC iterations is 254390.

TABLE S.3. The total numbers of walkers, reported as percentages of the total walker populations at 80000 MC iterations, characterizing the $i$-FCIQMC propagations with $\delta\tau = 0.0001$ a.u. that were needed to generate the CC($P$) and CC($P$;$Q$) results for cyclobutadiene reported in Table V of the main text.

| MC Iterations | X $^1B_{1g}$ | A $^3A_{2g}$ |
|---|---|---|
| 0 | 0.00[a] | 0.00[a] |
| 2000 | 0.00 | 0.00 |
| 4000 | 0.01 | 0.02 |
| 6000 | 0.02 | 0.04 |
| 8000 | 0.03 | 0.07 |
| 10000 | 0.05 | 0.09 |
| 20000 | 0.16 | 0.28 |
| 50000 | 3.81 | 4.93 |
| 80000 | 100[b] | 100[c] |

[a] The initial walker population, meaning 1500 walkers on the RHF (X $^1B_{1g}$ state) and ROHF (A $^3A_{2g}$ state) reference determinants.
[b] The total number of walkers at 80000 MC iterations is 8457504823.
[c] The total number of walkers at 80000 MC iterations is 4067481034.

TABLE S.4. The total numbers of walkers, reported as percentages of the total walker populations at 80000 MC iterations, characterizing the $i$-CISDTQ-MC propagations with $\delta\tau = 0.0001$ a.u. that were needed to generate the CC($P$) and CC($P$;$Q$) results for the cyclopentadienyl cation reported in Table VI of the main text.

| MC Iterations | X $^3A_2'$ | A $^1E_2'$ |
|---|---|---|
| 0 | 0.00[a] | 0.00[a] |
| 2000 | 0.01 | 0.00 |
| 4000 | 0.03 | 0.02 |
| 6000 | 0.06 | 0.05 |
| 8000 | 0.11 | 0.09 |
| 10000 | 0.16 | 0.13 |
| 20000 | 0.62 | 0.54 |
| 50000 | 13.20 | 15.73 |
| 80000 | 100[b] | 100[c] |

[a] The initial walker population, meaning 1500 walkers on the ROHF (X $^3A_2'$ state) and RHF (A $^1E_2'$ state) reference determinants.
[b] The total number of walkers at 80000 MC iterations is 7867091953.
[c] The total number of walkers at 80000 MC iterations is 11371381724.

TABLE S.5. The total numbers of walkers, reported as percentages of the total walker populations at 80000 MC iterations, characterizing the *i*-CISDTQ-MC propagations with $\delta\tau = 0.0001$ a.u. that were needed to generate the CC($P$) and CC($P$;$Q$) results for trimethylenemethane reported in Table VII of the main text.

| MC Iterations | X $^3A_2'$ | B $^1A_1$ |
|---|---|---|
| 0 | 0.00[a] | 0.00[a] |
| 2000 | 0.01 | 0.01 |
| 4000 | 0.06 | 0.05 |
| 6000 | 0.14 | 0.11 |
| 8000 | 0.24 | 0.18 |
| 10000 | 0.34 | 0.26 |
| 20000 | 1.09 | 0.93 |
| 50000 | 14.60 | 15.05 |
| 80000 | 100[b] | 100[c] |

[a] The initial walker population, meaning 1500 walkers on the ROHF (X $^3A_2'$ state) and RHF (B $^1A_1$ state) reference determinants.
[b] The total number of walkers at 80000 MC iterations is 2363904677.
[c] The total number of walkers at 80000 MC iterations is 3543757954.
